# Supplementary material for: DCAC: Dynamic Class-Aware Cache Creates Stronger Out-of-Distribution Detectors
Source: arXiv:2601.12468 source file (2026-01-18)
Supplement: Supplementary file 1 [file appendix.tex]

\clearpage
\newpage
\appendix
\begin{strip}
\section*{\huge Supplementary Material for DCAC: Dynamic Class-Aware Cache Creates Stronger Out-of-Distribution Detectors}
\end{strip}
\setcounter{secnumdepth}{2} %May be changed to 1 or 2 if section numbers are desired.

\section{Details of Datasets}
 % 子章节编号为 A.1, A.2, ...
\subsection{ImageNet Benchmark}
\paragraph{ImageNet-1K}~\cite{deng2009imagenet} is a large-scale image classification benchmark containing over 1.2 million training images and 50,000 validation images, spanning 1000 object classes. The images are collected from various real-world scenes and cover a wide range of object types, including animals, plants, vehicles, and household items. In our study, we use the validation set of ImageNet-1K (50000 images) as the in-distribution (ID) dataset.

\paragraph{iNaturalist}~\cite{van2018inaturalist} is a dataset containing images of the natural world, comprising 13 superclasses and 5089 subclasses that cover plants, insects, birds, mammals, and more. In our work, we adopt a subset of iNaturalist curated in the MCM~\cite{ming2022delving} containing 110 plant classes to avoid any overlap with the classes in ImageNet-1K, consisting of 10000 images. 

\paragraph{Places}~\cite{zhou2017places} is a large-scale dataset of scene photographs, encompassing labeled images across diverse semantic classes organized into three macro-classes: indoor, nature, and urban. In our work, we adopt a subset of Places curated in the MCM to avoid any overlap with the classes in ImageNet-1K, consisting of 10000 images.

\paragraph{SUN}~\cite{xiao2010sun} is a comprehensive scene recognition dataset comprising 397 carefully curated classes for benchmarking scene recognition algorithms, and a total of 899 classes spanning a broad spectrum of indoor, urban, and natural environments, with or without human presence. In our work, we adopt a subset of SUN curated in the MCM to avoid any overlap with the classes in ImageNet-1K, consisting of 10000 images.

\paragraph{Textures}~\cite{cimpoi2014describing} is a dataset comprising 5640 images of textures and abstract patterns, organized into 47 classes based on human perceptual similarity. As none of its classes overlap with ImageNet-1K, the entire dataset was used as OOD dataset.

\paragraph{NINCO}~\cite{bitterwolf2023ninco} is a dedicated OOD evaluation dataset designed to address limitations in ImageNet‑1K benchmarks. It comprises 64 OOD classes and a total of 5879 images, each manually inspected to ensure no overlap with any ImageNet‑1K class. The images were sourced from multiple datasets and newly scraped data, rigorously cleaned to guarantee the absence of ID objects.

\paragraph{SSB‑hard}~\cite{vaze2022openset} is the hard split of the Semantic Shift Benchmark (SSB), specifically designed for evaluating out‑of‑distribution detection under challenging semantic shifts. It comprises 49000 images sampled from 980 classes in ImageNet‑21K deliberately excluded from ImageNet‑1K . These classes are visually and semantically similar to the in‑distribution classes, making SSB‑hard a rigorous benchmark for hard‑OOD detection.

\subsection{CIFAR benchmark}
\paragraph{CIFAR-10 and CIFAR-100}~\cite{krizhevsky2009learning} are widely-used benchmark datasets in machine learning and computer vision research, originally derived from the 80 Million Tiny Images collection. CIFAR-10 consists of 60000 $32\times32$ color images evenly divided into 10 object classes (such as airplane, cat, dog, truck), with 6000 images per class: 50000 for training and 10000 for testing. CIFAR-100 extends this to 100 fine-grained classes, grouped into 20 superclasses, maintaining the same total image count: 60000 images (500 training, 100 testing per class), all at the same resolution and color depth.

\paragraph{SVHN (Street View House Numbers)}~\cite{SVHN} is a real-world dataset consisting of digit images cropped from Google Street View photographs of house numbers. It contains natural scene images with varying illumination, backgrounds, and digit positions. In our study, we use the complete SVHN test set, comprising 26032 images, as out-of-distribution (OOD) examples for evaluation.

\paragraph{LSUN (Large-scale Scene Understanding)}~\cite{LSUN} is a dataset designed for scene recognition, containing images of diverse environments such as bedrooms, houses, living rooms, and classrooms. LSUN\_C and LSUN\_R are derived variants obtained through cropping and resizing operations on the original images. For our evaluation, we randomly selected 10000 images from each of LSUN\_C and LSUN\_R to serve as out-of-distribution (OOD) examples.

\paragraph{Places365}~\cite{zhou2017places} is a large-scale dataset containing images classified to 365 distinct scene classes. The official test set includes 900 images per class. For our evaluation, we randomly selected 100 images from each class, providing a representative subset to assess the performance of algorithms across the diverse scene types in the Places365 dataset.

\paragraph{Texture}~\cite{cimpoi2014describing} comprises 5640 images of textures and abstract patterns, organized into 47 classes based on human perceptual attributes. As there is no class overlap with CIFAR, we employ the entire dataset.

\paragraph{iSUN}~\cite{iSUN} dataset is a large-scale eye-tracking dataset comprising 20608 natural scene images sourced from the SUN database. For our study, we selected 8925 images from iSUN that have no conceptual overlap with CIFAR, using them as out-of-distribution examples. These images offer distinct visual content, enabling performance evaluation beyond the scope of CIFAR.
\section{Details of Baseline Methods}
 % 子章节编号为 B.1, B.2, ...
\subsection{UniModal OOD Detection Methods}
\paragraph{Maximum Softmax Probability (MSP).}
Hendrycks \& Gimpel~ introduced the MSP score\cite{hendrycks2016baseline} to distinguish between in-distribution (ID) and out-of-distribution (OOD) samples. For a pre-trained model $f$, the MSP score is defined as:
{
\begin{align}
S_{\text{MSP}}(x; f)
&= \max_{c \in \{1, \dots, C\}} P(y = c \mid x; f) \notag \\
&= \max\bigl(\mathrm{softmax}(f(x))\bigr),
\end{align}
}where $x$ is the input sample, $C$ is the number of known classes, $\mathrm{softmax}(f(x))$ outputs the probability distribution over the $C$ classes. A higher MSP indicates greater confidence that $x$ belongs to a known class (ID), while a lower MSP suggests the sample may be OOD.
\paragraph{Energy.} Following the method in~\cite{liu2020energy}, the energy of the predicted logits is used to distinguish between ID and OOD samples. The energy score is defined as:
{
\begin{equation}
S_{\mathrm{Energy}}(x; f) = -T \log \sum_{c=1}^{C} \exp\left( \frac{f(x)_c}{T} \right),
\end{equation}
}where \(T\) is a temperature scaling parameter, and \(f(x)_c\) denotes the logit corresponding to class \(c\). A lower energy score implies a higher confidence that the input sample is from the ID distribution. In all our experiments, we set \(T = 1.0\) as recommended.
\paragraph{ReAct}\cite{sun2021react} is a lightweight post‑hoc method that mitigates overconfidence on OOD data by truncating large internal activations. Specifically, for the penultimate layer activations $h = [h_1, \dots, h_m]$:
{
\begin{equation}
\bar{h}_i = \min(h_i, c) \quad \text{for } i = 1, \dots, m,
\end{equation}
}where the threshold $c$ is set at the $p$-th percentile of in-distribution activations. The rectified vector $\bar{h}$ is then used for any standard OOD score (e.g., MSP or Energy). In all our experiments, we set $p=90$ and use energy score as a score function.
\paragraph{DICE}\cite{sun2022dice} is a simple yet effective post‑hoc sparsification approach that enhances OOD detection by masking irrelevant weights in the classifier layer. Let \(W \in \mathbb{R}^{C \times m}\) be the weight matrix of the final linear layer. DICE selects only the top‑\(q\) most contributive weights per class and zeros out the rest, yielding a sparse weight matrix \(W_{\text{DICE}}\). The resultant logits are:
{
\begin{equation}
f_{\text{DICE}}(x) = W_{\text{DICE}}\, h(x) + b,
\end{equation}
}where \(h(x)\) is the penultimate layer activation and \(b\) the bias. These sparse logits are then fed into standard scoring functions (e.g., MSP or Energy). In all our experiments, we set $q=30$ and use energy score as a score function.
\paragraph{ASH}\cite{djurisic2023extremely} is an ultra-simple, post-hoc method for OOD detection that manipulates activations in a late hidden layer. At inference time, a large fraction $p\%$ of the lowest activations are pruned, and the remaining ones are either uniformly scaled up (ASH‑S) or replaced with a constant value (ASH‑B). The modified activations are then passed through the rest of the network, and the resulting logits are used with standard scoring functions (e.g., MSP or Energy). In our experiments, we select ASH-B as baseline, we follow the recommended settings: we apply Energy scoring with $p=90$.
\paragraph{OptFS}~\cite{zhao2024towards} formulate feature shaping as an optimization problem and derive a piecewise‑constant shaping mask applied to penultimate layer features. Let $L(x) = W\cdot F(x) + B$ be the pre-trained logit, where \(F(x) \in \mathbb{R}^m\) is the feature vector and \(W \in \mathbb{R}^{C\times m}, B\in\mathbb{R}^C\) are classifier parameters. OptFS introduces a learned mask \(\theta \in \mathbb{R}^m\) such that
{
\begin{align}
&\tilde{F}(x) = \theta \odot F(x), \\
&L_{\mathrm{OptFS}}(x) = W\cdot (\tilde{F}(x)) + B,
\end{align}
}where \(\theta\) is piecewise‑constant: feature values are partitioned into \(K\) bins, each assigned a constant scaling factor. The optimal \(\theta\) is obtained in closed form using only ID data. In our experiments, we set $K=100$.
\paragraph{CADRef}~\cite{ling2025cadref} extend CARef by decomposing the relative feature error into positive and negative parts aligned with model weights, and scaling them via logit-based scores. Given:
\begin{align}
E(x) = \frac{\|F(x) - \mu_{T(x)}\|_1}{\|F(x)\|_1}, \\
\text{Score}_{\mathrm{CARef}}(x) = -E(x).
\end{align}
they define:
{
\begin{align}
    E_p(x) = \frac{\sum_{i:\,w_i^{c^*}F_i(x)>0} |F_i(x)-\mu_i^{c^*}|}{\|F(x)\|_1}, \\
E_n(x) = \frac{\sum_{i:\,w_i^{c^*}F_i(x)\le0} |F_i(x)-\mu_i^{c^*}|}{\|F(x)\|_1}.
\end{align}
}
Finally, the CADRef score is computed as:
{
\begin{equation}
\text{Score}_{\mathrm{CADRef}}(x)
= -\left(\frac{E_p(x)}{S_{\mathrm{logit}}(x)} + E_n(x)\cdot S_{\mathrm{logit}}^{\mathrm{mean}}\right),
\end{equation}
}where \(S_{\mathrm{logit}}(x)\) can be any logit-based function (e.g., Energy), and \(S_{\mathrm{logit}}^{\mathrm{mean}}\) is the mean logit score on ID data. In our experiments, we use energy score as logit-based function.
\subsection{VLM-based OOD Detection Methods}
\paragraph{MCM (Maximum Concept Matching)} is a simple yet effective zero‑shot method that computes OOD scores by aligning visual embeddings with textual class concepts using a pre‑trained vision‑language model like CLIP. Given an input $x'$ and ID class set $\mathcal{Y}_{\mathrm{in}}$ with textual embeddings $T_i$, the MCM score is:
{
\begin{equation}
\small
S_{\mathrm{MCM}}(x'; \mathcal{Y}_{\mathrm{in}}, \mathcal{T}, \mathcal{I}) 
= \max_{i=1,\dots,K} \frac{\exp(s_i(x')/\tau)}{\sum_{j=1}^K \exp(s_j(x')/\tau)},
\end{equation}
}where $s_i(x') = \mathrm{cosine}(E_v(x'), T_i)$ is the similarity for class $i$, $K = |\mathcal{Y}_{\mathrm{in}}|$, and $\tau$ is the softmax temperature. Samples with high $S_{\mathrm{MCM}}$ indicate strong alignment with one ID concept (likely ID), while low scores suggest OOD inputs. In our experiments, all the fine-tuning methods, like CoOp, LoCoOp, SCT, and OspCoOp, use MCM as their scoring function.
\paragraph{CSP (Conjugated Semantic Pool)} is a zero-shot OOD detection method that enriches the semantic anchor pool with adjective-decorated superclass labels to better separate in-distribution (ID) and out-of-distribution (OOD) samples. Let $h = E_v(x)$ be the image embedding from a vision-language model, $\{e_1, \dots, e_K\}$ be the textual embeddings of ID concepts, $\{\tilde{e}_1, \dots, \tilde{e}_M\}$ be the textual embeddings of OOD anchors, $\tau$ be the temperature scaling factor. The CSP score is computed as:
{
\begin{equation}
\small
S(x) = 
\frac{
\sum\limits_{i=1}^{K} \exp\left(\cos(h, e_i)/\tau\right)
}{
\sum\limits_{i=1}^{K} \exp\left(\cos(h, e_i)/\tau\right)
+ \sum\limits_{j=1}^{M} \exp\left(\cos(h, \tilde{e}_j)/\tau\right)
}.
\end{equation}
}

In CSP, we calibrate only the similarity between the visual features of test samples and the ID concepts.
\paragraph{Local‑Prompt} is a few-shot OOD detection framework built upon CLIP, which leverages both global and regional information through prompt learning. To better capture fine-grained features, the authors introduce a Regional-MCM score, which extends global MCM by aggregating the top‑$k$ most confident patch-level predictions and explicitly considering negative prompts:
\begin{align}
S_{\mathrm{pos}} =& \sum\limits_{j=1}^C \exp\left( \mathrm{sim}(z_h^l, t_j)/T \right),  \\
S_{\mathrm{neg}} =& \sum\limits_{j=1}^{N_{\mathrm{neg}}} \exp\left( \mathrm{sim}(z_h^l, \hat{t}_j)/T \right), \\
S_{\mathrm{Region}}=& \mathcal{T}_k^{\mathrm{mean}} \Bigg\{ 
\frac{
\exp\left( \mathrm{sim}(z_h^l, t_i)/T \right)
}{
 S_{\mathrm{pos}} + S_{\mathrm{neg}}   
}
\Bigg\}, \\
S_{\mathrm{R\text{-}MCM}}(x) 
&= S_{\mathrm{MCM}}(x)+ S_{\mathrm{Region}},
\end{align}
where $S_{\mathrm{MCM}}(x)$ is global MCM score, $\mathcal{T}_k^{\mathrm{mean}}(\cdot)$ is mean of top‑$k$ regional values, $t_j$ is ID textual embeddings, $\hat{t}_j$ is negative prompts, $z_h^l$ is visual features of spatial patch $h$, $T$ is temperature parameter. We only calibrate the MCM score. 
\paragraph{CMA}\cite{lee2025concept} is a zero-shot OOD detection framework that introduces neutral prompt into CLIP concept matching using a vector‑triangle relational structure. Given $
\{c_1, \dots, c_N\} \quad(\text{ID labels}),\quad
\{\hat{c}_1, \dots, \hat{c}_N\} \quad(\text{neutral agents}),$
image feature \(v = E_v(x)\), and similarity function \(\mathrm{sim}(\cdot,\cdot)\), CMA selects:$\hat{y} = \arg\max_i \mathrm{sim}(v, c_i),$
and computes the CMA score:

\begin{align}
S_{\mathrm{ID}} &=
\sum_{i=1}^N \exp\!\bigl(\mathrm{sim}(v, c_i)/\tau\bigr), \\
S_{\mathrm{Neutral}} &=
\sum_{i=1}^N \exp\!\bigl(\mathrm{sim}(v, c_i)/\tau\bigr), \\
S_{\mathrm{CMA}}(x) &=
\frac{\exp\!\bigl(\mathrm{sim}(v, \hat{c}_{\hat{y}})/\tau\bigr)}
{S_{\mathrm{ID}}+S_{\mathrm{Neutral}}}.
\end{align}

We also calibrate the similarity between the ID logits only.

\section{Details of Hyperparameter Configurations}
\label{hyper_config}
\begin{table}[!ht]
\centering
\small
\begin{tabular}{llcccc}
\toprule
\textbf{Architecture} & \textbf{Method} & $\alpha$ & $\beta$ & $k$ & $m$ \\
\midrule
\multirow{9}{*}{ResNet50} 
    & MSP & 0.9 & 95 & 20 & 20 \\
    & ODIN & 0.9 & 95 & 20 & 20 \\
    & Energy  & 0.9 & 95 & 20 & 20 \\
    & ReAct  & 1.0 & 99 & 20 & 20 \\
    & MaxLogits & 0.9 & 95 & 20 & 20 \\
    & DICE & 1.0 & 99 & 20 & 20 \\
    & ASH-S  & 0.05 & 95 & 20 & 20 \\
    & OptFs & 1.0 & 99 & 20 & 20 \\
    & CADRef & 0.9 & 95 & 20 & 20 \\
\midrule
\multirow{10}{*}{CLIP-B/16} 
    & MCM & 0.9 & 95 & 20 & 20 \\
    & CoOp & 0.9 & 95 & 20 & 20 \\
    & LoCoOp & 0.9 & 95 & 20 & 20 \\
    & NegLabel & 0.9 & 95 & 20 & 20 \\
    & SCT & 0.9 & 95 & 20 & 20 \\
    & CSP & 0.9 & 95 & 20 & 20 \\    
    & CMA & 0.9 & 95 & 20 & 20 \\
    & Local-Prompt & 0.9 & 95 & 20 & 20 \\
    & OODD  & 0.9 & 95 & 20 & 20 \\  
    & OSPCoOp & 0.9 & 95 & 20 & 20 \\
    
\bottomrule
\end{tabular}
\caption{Detailed hyperparameter configuration for each baseline method.}
\label{tab:hyper_config}
\end{table}

 % 子章节编号为 D.1, D.2, ...
\section{Further Analysis}
\label{further_analysis}
\subsection{Visual similarity comparison}
\label{vis_sim_compare}
We compute and analyze the average visual similarity on both ResNet50 and CLIP-B/16 between unconfident OOD samples predicted as each ID class and two groups: (1) overconfident OOD samples assigned high confidence to the same class, and (2) ID samples predicted to the same class. As shown in Fig. \ref{fig:vis_sim_clip} and Fig. \ref{fig:vis_sim_resnet}, the average similarity between the two types of OOD samples is higher than that between unconfident OOD samples and ID samples. Moreover, we found that this phenomenon is more pronounced in the CLIP-B/16. The underlying reason is that overconfident OOD samples in CLIP are entirely dissimilar to ID samples at the level of visual features. In contrast, in unimodal models, overconfident OOD samples often share certain visual similarities,such as background,with the ID samples.

\begin{figure*}[!ht]
\centering
\includegraphics[width=\textwidth]{CameraReady/LaTeX/images/un_cosine_similarity_boxplots_2x2_clip.pdf} % Reduce the figure size so that it is slightly narrower than the column.
\caption{CLIP-B/16: Visual similarity comparison on ImageNet-1K far-OOD benchmark.}
\label{fig:vis_sim_clip}
\end{figure*}

\begin{figure*}[!ht]
\centering
\includegraphics[width=\textwidth]{CameraReady/LaTeX/images/un_cosine_similarity_boxplots_2x2_resnet.pdf} % Reduce the figure size so that it is slightly narrower than the column.
\caption{ResNet50: Visual similarity comparison on ImageNet-1K far-OOD benchmark.}
\label{fig:vis_sim_resnet}
\end{figure*}

\onecolumn  % 切换到单列模式
\clearpage
\newpage

\begin{figure}[!ht]
\centering
\includegraphics[width=\textwidth]{CameraReady/LaTeX/images/msp_visualize.pdf} % Reduce the figure size so that it is slightly narrower than the column.
\captionsetup{skip=2pt}  % 仅对这一幅图起效
\caption{Visualization of test samples predicted as the same class by ResNet50.}
\label{fig:vis_cache_res}
\end{figure}

\begin{figure}[!ht]
\centering
\includegraphics[width=\textwidth]{CameraReady/LaTeX/images/mcm_visualize.pdf} % Reduce the figure size so that it is slightly narrower than the column.
\captionsetup{skip=2pt}  % 仅对这一幅图起效
\caption{Visualization of test samples predicted as the same class by CLIP-B/16.}
\label{fig:vis_cache_clip}
\end{figure}
\twocolumn

\subsection{Visualize of the cache samples}
\label{vis_cached_samples}
As shown in Fig. \ref{fig:vis_cache_res}, the visualization includes three types of samples: true ID samples, overconfident OOD samples, and unconfident OOD samples. All three share similar background content; however, only the true ID samples contain meaningful foreground objects. In contrast, the OOD samples consist mainly of background. Although the model assigns high confidence to some of these backgrounds, they remain visually similar to low-confidence OOD samples.

As shown in Fig. \ref{fig:vis_cache_clip}, among these samples, the ID and OOD samples are highly dissimilar in visual features. However, some OOD samples exhibit high similarity to the text embeddings of the predicted ID class. In contrast, the OOD samples themselves share more similar visual characteristics with each other, but entirely unsimiliar with ID samples.
\subsection{Comparison of Calibration Performance on ID and OOD Samples}
\label{cal_performance}
\begin{figure}[h]
\centering
\includegraphics[width=0.48\textwidth,height=0.35\textwidth]{CameraReady/LaTeX/images/fuzzy_logits_difference.pdf} % Reduce the figure size so that it is slightly narrower than the column.
\caption{The mean difference between the $\mathbf{z_{\mathrm{cache}}}$ of OOD samples and those of ID samples. The results demonstrate that this difference is consistently negative, suggesting that calibration imposes a stronger correction on OOD samples, thereby alleviating their overconfident predictions.}
\label{fig:z_cal}
\end{figure}
\noindent The calibrated logits of our method are expressed as:
\begin{equation}
% \small
\mathbf{z}_{\mathrm{cache}} = -\mathbf{P}_{k} \mathbf{F}^\intercal
\mathbf{f}_{\mathrm{test}} ,
\end{equation}
assuming $\mathbf{P}_{k}$ is fixed, we focus only on the last two terms. The last two terms represent the cosine similarity between the visual features of the test sample and those of the cached samples.
If the visual similarity between them is high, it indicates that the resulting logits will generally have larger values. OOD samples often exhibit high similarity with cached samples that belong to the predicted class or have high predicted probabilities for that class. As a result,the values of these classes in $\mathbf{z_{\mathrm{cache}}}$ are relatively small. Therefore, the final logits of overconfident classes can be effectively reduced. For ID samples, their visual similarity with cached samples is relatively low. As a result, the values in $\mathbf{z_{\mathrm{cache}}}$ are relative large and the final predictions are less affected. The results in Fig.\ref{fig:z_cal} confirm our analysis.

\subsection{Calibration effectiveness}
\label{Calibration_effectiveness}
We compared the KL divergence between the predicted probability distribution and the uniform distribution before and after calibration, as shown in Table \ref{tab:kl_divergence}. The calibration effectively reduces overconfidence in OOD samples, where the  KL divergence of ID samples remains largely unchanged, whereas the distribution of OOD samples becomes more uniform after calibration. Fig.\ref{fig:sun_mcm}, Fig.\ref{fig:places_mcm} and Fig.\ref{fig:dtd_mcm} show the changes in MCM scores on SUN, Places, and Textures before and after calibration.

\begin{table}[htbp]
\centering
\small
\setlength{\tabcolsep}{1mm}
\begin{tabular}{lcccc}
\hline

\multirow{2}{*}{\begin{tabular}[c]{@{}c@{}}{\textbf{Metric}}\end{tabular}} 
\textbf{} & \multicolumn{4}{c}{\textbf{OOD Dataset}} \\ \cline{2-5} 
& \textbf{iNaturalist} & \textbf{SUN} & \textbf{Places} & \textbf{Textures} \\
\hline
KL (ID Original)$\uparrow$   & 7.17 & 7.17 & 7.17 & 7.17 \\
KL (ID Calibrated)$\uparrow$  & \textbf{7.20} & \textbf{7.20} & \textbf{7.19} & \textbf{7.18} \\
KL (OOD Original)$\downarrow$  & 3.30 & 3.42 & 3.64 & 4.20 \\
KL (OOD Calibrated)$\downarrow$ & \textbf{2.41} & \textbf{2.43} & \textbf{2.82} & \textbf{3.25} \\
\hline
\end{tabular}
\caption{Average KL divergence between the predicted and uniform distributions for ID and OOD data across datasets, before and after calibration of CLIP-B/16. }
\label{tab:kl_divergence}
\end{table}

\begin{figure}[h]
    \centering
    \includegraphics[width=0.45\textwidth]{CameraReady/LaTeX/images/sun_calibrated_visualized.pdf}
    \caption{Comparison of the MCM score distribution on SUN before and after calibration.}
    \label{fig:sun_mcm}
\end{figure}
\begin{figure}[h]
    \centering
    \includegraphics[width=0.45\textwidth]{CameraReady/LaTeX/images/places_calibrated_visualized.pdf}
    \caption{Comparison of the MCM score distribution on Places before and after calibration.}
    \label{fig:places_mcm}
\end{figure}
\begin{figure}[!h]
    \centering
    \includegraphics[width=0.45\textwidth]{CameraReady/LaTeX/images/dtd_calibrated_visualized.pdf}
    \caption{Comparison of the MCM score distribution on Textures before and after calibration.}
    \label{fig:dtd_mcm}
\end{figure}

\clearpage
\newpage
\onecolumn  % 切换到单列模式
\section{Detailed Experimental Results}
\label{detail_exp_results}

\begin{table}[!htbp]
\fontsize{8}{9}\selectfont % 设置字体大小为 7pt，行距为 9pt
% \small
\centering
\setlength{\tabcolsep}{1mm}
\begin{tabular}{@{}llllllllllll@{}} \toprule
    {\multirow{2.5}{*}{\begin{tabular}[c]{@{}c@{}} Method\end{tabular}}}   
    & \multicolumn{2}{c}{iNaturalist} 
    & \multicolumn{2}{c}{SUN} 
    & \multicolumn{2}{c}{Places}  
    & \multicolumn{2}{c}{Texture} 
    & \multicolumn{2}{c}{\textbf{Average}} \\ 
    \cmidrule(lr){2-3} \cmidrule(lr){4-5} \cmidrule(lr){6-7} \cmidrule(lr){8-9} \cmidrule(lr){10-11}
    & FPR95$\downarrow$ & AUROC$\uparrow$ 
    & FPR95$\downarrow$ & AUROC$\uparrow$ 
    & FPR95$\downarrow$ & AUROC$\uparrow$ 
    & FPR95$\downarrow$ & AUROC$\uparrow$ 
    & FPR95$\downarrow$ & AUROC$\uparrow$  \\ \midrule

    MSP & 52.73 & 88.42 & 68.58 & 81.75 & 71.59 & 80.63 & 66.15 & 80.46 & 64.76 & 82.82 \\
    \textbf{MSP+Ours} & \textbf{24.84$\pm$0.40} & \textbf{95.09$\pm$0.03} & \textbf{36.68$\pm$0.31} & \textbf{91.46$\pm$0.08} & \textbf{46.78$\pm$0.57} & \textbf{88.51$\pm$0.07} & \textbf{50.83$\pm$0.12} & \textbf{85.99$\pm$0.06} & \textbf{39.78$\pm$0.18} & \textbf{90.26$\pm$0.03} \\
    \cmidrule(lr){1-11}
    ODIN & 52.33 & 87.00 & 53.49 & 86.57 & 58.64 & 85.30 & 46.08 & 86.51 & 52.64 & 86.35 \\
    \textbf{ODIN+Ours} & \textbf{19.18$\pm$0.12} & \textbf{96.62$\pm$0.04} & \textbf{28.19$\pm$0.15} & \textbf{94.35$\pm$0.05} & \textbf{39.48$\pm$0.25} & \textbf{91.24$\pm$0.06} & \textbf{39.54$\pm$0.23} & \textbf{90.63$\pm$0.04} & \textbf{\textbf{31.60$\pm$0.06}} & \textbf{93.21$\pm$0.02} \\
    \cmidrule(lr){1-11}
    Energy  & 53.96 & 90.59 & 58.28 & 86.73 & 65.43 & 84.12 & 52.3 & 86.73 & 57.49 & 87.04 \\
    \textbf{Energy+Ours} & \textbf{31.15$\pm$0.46} & \textbf{94.93$\pm$0.07} & \textbf{37.27$\pm$0.44} & \textbf{92.86$\pm$0.07} & \textbf{48.45$\pm$0.26} & \textbf{89.77$\pm$0.07} & \textbf{47.16$\pm$0.76} & \textbf{89.29$\pm$0.08} & \textbf{\textbf{41.01$\pm$0.27}} & \textbf{91.71$\pm$0.02} \\
    \cmidrule(lr){1-11}
    MaxLogits  & 50.77 & 91.14 & 60.39 & 86.43 & 66.03 & 84.03 & 54.91 & 86.38 & 58.03 & 87.00 \\
    \textbf{MaxLogits+Ours} & \textbf{23.47$\pm$0.19} & \textbf{95.90$\pm$0.06} & \textbf{32.88$\pm$0.47} & \textbf{93.42$\pm$0.06} & \textbf{43.91$\pm$0.35} & \textbf{90.33$\pm$0.07} & \textbf{45.11$\pm$0.10} & \textbf{89.48$\pm$0.08} & \textbf{\textbf{36.34$\pm$0.14}} & \textbf{92.28$\pm$0.02} \\
    \cmidrule(lr){1-11}
   ReAct  & 19.55 & 96.39 & 24.01 & 94.41 & 33.45 & 91.93 & 45.83 & 90.45 & 30.71 & 93.30 \\
    \textbf{ReAct+Ours} & \textbf{7.71$\pm$0.28} & \textbf{98.39$\pm$0.06} & \textbf{13.90$\pm$0.03} & \textbf{96.74$\pm$0.02} & \textbf{25.43$\pm$0.14} & \textbf{93.90$\pm$0.01} & \textbf{36.05$\pm$0.37} & \textbf{92.85$\pm$0.12} & \textbf{\textbf{20.77$\pm$0.16}} & \textbf{95.47$\pm$0.02} \\
    \cmidrule(lr){1-11}
    DICE   & 26.63 & 94.51 & 36.48 & 90.91 & 47.98 & 87.64 & 32.58 & 90.44  & 35.92 & 90.88 \\
    \textbf{DICE+Ours} & \textbf{17.46$\pm$0.18} & \textbf{96.56$\pm$0.04} & \textbf{25.43$\pm$0.02} & \textbf{94.24$\pm$0.02} & \textbf{38.17$\pm$0.25} & \textbf{90.91$\pm$0.07} & \textbf{28.88$\pm$0.12} & \textbf{91.95$\pm$0.04} & \textbf{27.49$\pm$0.06} & \textbf{93.42$\pm$0.01} \\
    \cmidrule(lr){1-11}
    ASH-S  & 11.49 & 97.87 & 27.96 & 94.02 & 39.83 & 90.98 & 11.97 & 97.6 & 22.81 & 95.12 \\
    \textbf{ASH-S+Ours} & \textbf{6.69$\pm$0.12} & \textbf{98.54$\pm$0.01} & \textbf{17.47$\pm$0.28} & \textbf{96.21$\pm$0.04} & \textbf{29.18$\pm$0.20} & \textbf{93.11$\pm$0.02}  & \textbf{11.70$\pm$0.25} & \textbf{97.74$\pm$0.01} & \textbf{16.26$\pm$0.10} & \textbf{96.40$\pm$0.01} \\
    \cmidrule(lr){1-11}
    OptFS & 16.79 & 96.88 & 35.31 & 93.13 & 44.78 & 90.42 & 23.08 & 95.74 & 29.99 & 94.04              \\
    \textbf{OptFS+Ours} & \textbf{6.86$\pm$0.17} & \textbf{98.53$\pm$0.02} & \textbf{18.14$\pm$0.21} & \textbf{96.12$\pm$0.01} & \textbf{29.42$\pm$0.34} & \textbf{93.07$\pm$0.01} & \textbf{16.75$\pm$0.13} & \textbf{96.99$\pm$0.02} & \textbf{17.79$\pm$0.04} & \textbf{96.18$\pm$0.01} \\
    \cmidrule(lr){1-11}
    CADRef & 16.08 & 96.9 & 39.23 & 91.26 & 51.12 & 87.8 & \textbf{12.60} & 97.14 & 29.76 & 93.28              \\
    \textbf{CADRef+Ours} & \textbf{10.43$\pm$0.15} & \textbf{97.98$\pm$0.02} & \textbf{26.19$\pm$0.31} & \textbf{94.83$\pm$0.05} & \textbf{39.09$\pm$0.49} & \textbf{91.59$\pm$0.04} & 13.20$\pm$0.08 & 97.14$\pm$0.01 & \textbf{22.22$\pm$0.23} & \textbf{95.38$\pm$0.01} \\
    \bottomrule
\end{tabular}
\caption{Compatibility experiments of our method combined with different OOD detection methods on ResNet50.}
\label{tab:comparison_rn50}
\end{table}

\begin{table*}[!ht]
\fontsize{8}{9}\selectfont % 设置字体大小为 7pt，行距为 9pt
% \small
\centering
\setlength{\tabcolsep}{1mm}
\begin{tabular}{@{}llllllllllll@{}} \toprule
    {\multirow{2.5}{*}{\begin{tabular}[c]{@{}c@{}} Method\end{tabular}}}   
    & \multicolumn{2}{c}{iNaturalist} 
    & \multicolumn{2}{c}{SUN} 
    & \multicolumn{2}{c}{Places}  
    & \multicolumn{2}{c}{Texture} 
    & \multicolumn{2}{c}{\textbf{Average}} \\ 
    \cmidrule(lr){2-3} \cmidrule(lr){4-5} \cmidrule(lr){6-7} \cmidrule(lr){8-9} \cmidrule(lr){10-11}
    & FPR95$\downarrow$ & AUROC$\uparrow$ 
    & FPR95$\downarrow$ & AUROC$\uparrow$ 
    & FPR95$\downarrow$ & AUROC$\uparrow$ 
    & FPR95$\downarrow$ & AUROC$\uparrow$ 
    & FPR95$\downarrow$ & AUROC$\uparrow$  \\ \midrule

    \multicolumn{11}{c}{\textbf{Zero-shot (no training required)}} \\
    MCM & 31.95 & 94.16 & 37.22 & 92.55 & 42.98 & 90.10 & 58.35 & 85.83 & 42.63 & 90.66 \\
    \textbf{MCM+Ours} & \textbf{7.39$\pm$0.23} & \textbf{98.27$\pm$0.02} & \textbf{17.56$\pm$0.09} & \textbf{96.65$\pm$0.06} & \textbf{29.62$\pm$0.54} & \textbf{93.05$\pm$0.01} & \textbf{42.43$\pm$0.55} & \textbf{90.72$\pm$0.10} & \textbf{24.25$\pm$0.27} & \textbf{94.67$\pm$0.01} \\
    \cmidrule(lr){1-11}
    GL-MCM & 17.42 & 96.44 & 30.75 & 93.44 & 37.62 & 90.63 & 55.20 & 85.54 & 35.25 & 91.51 \\
    \textbf{GL-MCM+Ours} & \textbf{5.14$\pm$0.05} & \textbf{98.76$\pm$0.01} & \textbf{16.46$\pm$0.18} & \textbf{96.56$\pm$0.04} & \textbf{27.77$\pm$0.11} & \textbf{92.93$\pm$0.01} & \textbf{44.98$\pm$0.28} & \textbf{88.34$\pm$0.09} & \textbf{23.58$\pm$0.02} & \textbf{94.14$\pm$0.01} \\
    \cmidrule(lr){1-11}
    CSP & 1.54 & 99.60 & 13.66 & 96.66 & 29.32 & 92.90 & 25.52 & 93.86 & 17.51 & 95.76 \\
    \textbf{CSP+Ours} & \textbf{1.20$\pm$0.02} & \textbf{99.62$\pm$0.01} & \textbf{10.18$\pm$0.03} & \textbf{97.58$\pm$0.01} & \textbf{25.29$\pm$0.16} & \textbf{93.94$\pm$0.02} & \textbf{20.62$\pm$0.12} & \textbf{95.27$\pm$0.03} & \textbf{\textbf{14.32$\pm$0.04}} & \textbf{96.60$\pm$0.01} \\
    \cmidrule(lr){1-11}
    OODD  & 2.22 & 99.36 & 21.49 & 95.01 & 44.76 & 87.10 & 30.69 & 93.27 & 24.79 & 93.69 \\
    \textbf{OODD+Ours} & \textbf{1.21$\pm$0.05} & \textbf{99.70$\pm$0.01} & \textbf{16.20$\pm$0.07} & \textbf{96.55$\pm$0.07} & \textbf{33.62$\pm$0.68} & \textbf{91.15$\pm$0.16} & \textbf{25.49$\pm$0.13} & \textbf{94.74$\pm$0.04} & \textbf{\textbf{19.13$\pm$0.26}} & \textbf{95.53$\pm$0.05} \\
    \cmidrule(lr){1-11}
   CMA  & 8.88 & 98.19 & 29.03 & 93.32 & 27.60 & 93.87 & 51.26 & 87.00 & 29.19 & 93.10 \\
    \textbf{CMA+Ours} & \textbf{2.36$\pm$0.06} & \textbf{99.45$\pm$0.01} & \textbf{13.10$\pm$0.07} & \textbf{97.33$\pm$0.06} & \textbf{20.71$\pm$0.08} & \textbf{95.37$\pm$0.02} & \textbf{36.29$\pm$0.21} & \textbf{92.41$\pm$0.09} & \textbf{\textbf{18.12$\pm$0.06}} & \textbf{96.14$\pm$0.02} \\
    \midrule
    \multicolumn{11}{c}{\textbf{finetuning based methods}} \\	
    CoOp   & 14.60 & 96.62 & 28.48 & 92.65 & 36.49 & 89.98 & 43.13 & 88.03  & 30.67 & 91.82 \\
    \textbf{CoOp+Ours} & \textbf{4.88$\pm$0.08} & \textbf{98.76$\pm$0.01} & \textbf{15.90$\pm$0.55} & \textbf{96.76$\pm$0.02} & \textbf{27.71$\pm$0.21} & \textbf{93.09$\pm$0.01} & \textbf{27.74$\pm$0.34} & \textbf{93.62$\pm$0.05} & \textbf{19.05$\pm$0.16} & \textbf{95.56$\pm$0.02} \\
    \cmidrule(lr){1-11}
    LoCoOp  & 16.05 & 96.86 & 23.44 & 95.07 & 32.87 & 91.98 & 42.28 & 90.19 & 28.66 & 93.52 \\
    \textbf{LoCoOp+Ours} & \textbf{4.38$\pm$0.08} & \textbf{98.79$\pm$0.01} & \textbf{12.45$\pm$0.21} & \textbf{97.35$\pm$0.03} & \textbf{24.09$\pm$0.15} & \textbf{93.81$\pm$0.02}  & \textbf{26.29$\pm$0.15} & \textbf{94.58$\pm$0.06} & \textbf{16.80$\pm$0.10} & \textbf{96.13$\pm$0.02} \\
    \cmidrule(lr){1-11}
    SCT & 13.94 & 95.86 & 20.55 & 95.33 & 29.86 & 92.24 & 41.51 & 89.06 & 26.47 & 93.37              \\
    \textbf{SCT+Ours} & \textbf{5.80$\pm$0.26} & \textbf{97.19$\pm$0.04} & \textbf{13.95$\pm$0.27} & \textbf{97.19$\pm$0.05} & \textbf{25.82$\pm$0.13} & \textbf{93.31$\pm$0.03} & \textbf{29.99$\pm$0.29} & \textbf{93.02$\pm$0.04} & \textbf{18.89$\pm$0.06} & \textbf{95.50$\pm$0.02} \\
    \cmidrule(lr){1-11}
    OSPCoOp & 15.25 & 97.13 & 18.26 & 96.74 & 25.74 & 94.01 & 41.26 & 91.13 & 25.13 & 94.75              \\
    \textbf{OSPCoOp+Ours} & \textbf{4.51$\pm$0.09} & \textbf{98.72$\pm$0.01} & \textbf{9.90$\pm$0.28} & \textbf{97.92$\pm$0.01} & \textbf{21.03$\pm$0.14} & \textbf{94.65$\pm$0.01} & \textbf{31.08$\pm$0.33} & \textbf{93.82$\pm$0.02} & \textbf{16.63$\pm$0.10} & \textbf{96.28$\pm$0.01} \\
    \cmidrule(lr){1-11}
    Local-Prompt & 8.71 & 98.10 & 23.97 & 94.85 & 32.50 & 92.32 & 47.93 & 89.04 & 28.27 & 93.58              \\
    \textbf{Local-Prompt+Ours} & \textbf{3.53$\pm$0.08} & \textbf{99.17$\pm$0.01} & \textbf{12.58$\pm$0.15} & \textbf{97.43$\pm$0.04} & \textbf{22.66$\pm$0.14} & \textbf{94.23$\pm$0.01} & \textbf{36.81$\pm$0.35} & \textbf{91.78$\pm$0.06} & \textbf{18.90$\pm$0.11} & \textbf{95.65$\pm$0.01} \\ 
    \bottomrule
\end{tabular}
\caption{Compatibility experiments of our method combined with different OOD detection methods on CLIP-B/16.}
\label{tab:comparison_b16}
\end{table*}

\begin{table}[t]
\centering
\small
% \setlength{\tabcolsep}{1mm} % <<< 控制列间距
% \resizebox{1\textwidth}{!}{%
    \begin{tabular}{@{}llllllll@{}} \toprule
        {\multirow{2.5}{*}{\begin{tabular}[c]{@{}c@{}} Backbone\end{tabular}}}  
        & {\multirow{2.5}{*}{\begin{tabular}[c]{@{}c@{}} Method\end{tabular}}}  
        & \multicolumn{2}{c}{NINCO} 
        & \multicolumn{2}{c}{SSB-hard} 
        & \multicolumn{2}{c}{\textbf{Average}} \\ 
        \cmidrule(lr){3-4} \cmidrule(lr){5-6} \cmidrule(lr){7-8}
        & 
        &  FPR95$\downarrow$ &  AUROC$\uparrow$ 
        &  FPR95$\downarrow$ &  AUROC$\uparrow$ 
        &  FPR95$\downarrow$ &  AUROC$\uparrow$  \\ 
        \midrule
    \multirow{16}{*}{ResNet} 
    & MSP & 75.94 & 79.97 & 84.54 & 72.16 & 80.24 & 76.07 \\
    & \textbf{MSP+Ours} & \textbf{70.58$\pm$0.53} & \textbf{82.61$\pm$0.13} & \textbf{74.49$\pm$0.09} & \textbf{77.38$\pm$0.08} & \textbf{72.58$\pm$0.53} & \textbf{79.99$\pm$0.10} \\
    \cmidrule(lr){2-8}
    & ODIN & 76.64 & 80.40 & 83.75 & 72.75 & 80.20 & 76.58 \\
    & \textbf{ODIN+Ours} & \textbf{71.98$\pm$0.66} & \textbf{82.96$\pm$0.18} & \textbf{70.25$\pm$0.05} & \textbf{80.39$\pm$0.07} & \textbf{71.12$\pm$0.31} & \textbf{81.67$\pm$0.12} \\
    \cmidrule(lr){2-8}
    & Energy & 77.63 & 79.69 & 83.87 & 72.35 & 80.75 & 76.02 \\
    & \textbf{Energy+Ours} & \textbf{77.21$\pm$0.13} & \textbf{81.12$\pm$0.11} & \textbf{75.29$\pm$0.59} & \textbf{77.86$\pm$0.07} & \textbf{76.25$\pm$0.36} & \textbf{79.49$\pm$0.06} \\
    \cmidrule(lr){2-8}
    & MaxLogits & 76.64 & 80.40 & 83.75 & 72.75 & 80.20 & 76.58 \\
    & \textbf{MaxLogits+Ours} & \textbf{73.23$\pm$0.22} & \textbf{82.08$\pm$0.17} & \textbf{73.16$\pm$0.04} & \textbf{78.45$\pm$0.08} & \textbf{73.20$\pm$0.09} & \textbf{80.27$\pm$0.12} \\
    \cmidrule(lr){2-8}
    & DICE & 74.09 & 77.52 & 81.06 & 72.82 & 77.58 & 75.17 \\
    & \textbf{DICE+Ours} & \textbf{72.42$\pm$0.21} & \textbf{78.78$\pm$0.07} & \textbf{72.87$\pm$0.31} & \textbf{77.62$\pm$0.12} & \textbf{72.64$\pm$0.16} & \textbf{78.20$\pm$0.07} \\
    \cmidrule(lr){2-8}
    & ReAct & \textbf{71.21} & \textbf{80.15} & 79.07 & 72.81 & 75.14 & 76.48 \\
    & \textbf{ReAct+Ours} & 72.49$\pm$0.26 & 79.84$\pm$0.08 & \textbf{77.60$\pm$0.15} & \textbf{74.25$\pm$0.02} & \textbf{75.05$\pm$0.21} & \textbf{77.04$\pm$0.03} \\
    \cmidrule(lr){2-8}
    & ASH & 65.02 & 82.77 & 82.53 & 70.49 & 73.75 & 76.63 \\
    & \textbf{ASH+Ours} & \textbf{63.36$\pm$0.25} & \textbf{83.89$\pm$0.04} & \textbf{69.95$\pm$0.24} & \textbf{81.32$\pm$0.07} & \textbf{66.65$\pm$0.09} & \textbf{82.60$\pm$0.02} \\
    \cline{2-8}
    & CADRef & 64.89 & 85.36 & 78.79 & 74.58 & 71.84 & 79.97 \\
    & \textbf{CADRef+Ours} & \textbf{63.64$\pm$0.36} & \textbf{85.46$\pm$0.01} & \textbf{74.32$\pm$0.16} & \textbf{78.71$\pm$0.09} & \textbf{68.98$\pm$0.12} & \textbf{82.08$\pm$0.04} \\
    \midrule
    \multirow{16}{*}{CLIP-B/16} 
    & MCM & 79.50 & 74.57 & 89.90 & 62.95 & 84.70 & 68.76 \\
    & \textbf{MCM+Ours} & \textbf{75.92$\pm$0.57} & \textbf{75.02$\pm$0.07} & \textbf{84.05$\pm$0.36} & \textbf{67.85$\pm$0.08} & \textbf{79.98$\pm$0.40} & \textbf{71.43$\pm$0.06} \\
    \cline{2-8}
    & CSP & 69.01 & 77.69 & 82.74 & 71.93 & 75.88 & 74.81 \\
    & \textbf{CSP+Ours} & \textbf{66.71$\pm$0.23} & \textbf{80.52$\pm$0.04} & \textbf{78.90$\pm$0.14} & \textbf{76.12$\pm$0.03} & \textbf{72.81$\pm$0.10} & \textbf{78.32$\pm$0.02} \\
    \cline{2-8}
    & CMA & 62.67 & 82.78 & 83.91 & 68.76 & 73.29 & 75.77 \\
    & \textbf{CMA+Ours} & \textbf{61.75$\pm$0.23} & \textbf{83.58$\pm$0.10} & \textbf{79.08$\pm$0.13} & \textbf{72.36$\pm$0.12} & \textbf{70.42$\pm$0.13} & \textbf{77.97$\pm$0.08} \\
    \cline{2-8}
    & CoOp & 78.27 & 73.58 & 87.92 & 64.10 & 83.10 & 68.84 \\
    & \textbf{CoOp+Ours} & \textbf{73.82$\pm$0.34} & \textbf{74.53$\pm$0.03} & \textbf{81.82$\pm$0.11} & \textbf{66.59$\pm$0.13} & \textbf{77.82$\pm$0.23} & \textbf{70.56$\pm$0.08} \\
    \cline{2-8}
    & LoCoOp & 78.27 & 73.58 & 87.92 & 64.10 & 83.10 & 68.84 \\
    & \textbf{LoCoOp+Ours} & \textbf{73.82$\pm$0.34} & \textbf{74.53$\pm$0.03} & \textbf{81.82$\pm$0.11} & \textbf{66.59$\pm$0.13} & \textbf{77.82$\pm$0.23} & \textbf{70.56$\pm$0.08} \\
    \cline{2-8}
    & SCT & 79.07 & 70.18 & 89.12 & 63.19 & 84.10 & 66.69 \\
    & \textbf{SCT+Ours} & \textbf{76.04$\pm$0.25} & \textbf{70.30$\pm$0.06} & \textbf{84.36$\pm$0.04} & \textbf{64.88$\pm$0.03} & \textbf{80.20$\pm$0.12} & \textbf{67.59$\pm$0.02} \\
    \cline{2-8}
    & Local-Prompt & 71.73 & 77.31 & 84.45 & 69.54 & 78.09 & 73.43 \\
    & \textbf{Local-Prompt+Ours} &\textbf{70.21$\pm$0.19} & \textbf{77.75$\pm$0.05} & \textbf{81.30$\pm$0.38} & \textbf{70.90$\pm$0.06} & \textbf{75.76$\pm$0.18} & \textbf{74.33$\pm$0.04} \\
    \cline{2-8}
    & OSPCoOp & 80.81 & 70.77 & 92.56 & 60.13 & 86.69 & 65.45 \\
    & \textbf{OSPCoOp+Ours} &\textbf{79.11$\pm$0.17} & \textbf{71.04$\pm$0.09} & \textbf{90.51$\pm$0.07} & \textbf{60.90$\pm$0.05} & \textbf{84.81$\pm$0.12} & \textbf{65.97$\pm$0.06} \\
    \bottomrule
\end{tabular}
% }
\caption{Comparison results on hard-OOD datasets}
\label{tab:comparison_hard}
\end{table}

\begin{table}[!ht]
\centering
\fontsize{7}{9}\selectfont % 设置字体大小为 7pt，行距为 9pt
\setlength{\tabcolsep}{1mm}
\begin{tabular}{clccccccccccccccc}
\toprule
\multirow{3}{*}{\begin{tabular}[c]{@{}c@{}}{Architecture}\end{tabular}} 
&\multirow{3}{*}{Method} & \multicolumn{8}{c}{OOD Datasets} & \multicolumn{2}{c}{\multirow{2}{*}{Average}} \\ \cline{3-10} 
&  & \multicolumn{2}{c}{iNaturalist} & \multicolumn{2}{c}{SUN} & \multicolumn{2}{c}{Textures} & \multicolumn{2}{c}{Places} \\
\cmidrule(lr){3-4} \cmidrule(lr){5-6} \cmidrule(lr){7-8} \cmidrule(lr){9-10} \cmidrule(lr){11-12}
& & FPR95$\downarrow$ & AUROC$\uparrow$ 
& FPR95$\downarrow$ & AUROC$\uparrow$ 
& FPR95$\downarrow$ & AUROC$\uparrow$ 
& FPR95$\downarrow$ & AUROC$\uparrow$ 
& FPR95$\downarrow$ & AUROC$\uparrow$ \\ 
\midrule
\multirow{2}{*}{\begin{tabular}[c]{@{}c@{}}DenseNet201\end{tabular}} 
    & MSP & 44.80 & 89.83 & 65.22 & 82.22 & 67.02 & 79.40 & 68.86 & 81.13 & 61.48 & 83.15 \\
    & \textbf{MSP+Ours} & \textbf{20.50$\pm$0.45} & \textbf{95.45$\pm$0.16} & \textbf{31.96$\pm$0.45} & \textbf{91.65$\pm$0.13} & \textbf{59.76$\pm$0.20} & \textbf{82.14$\pm$0.13} & \textbf{43.08$\pm$0.04} & \textbf{88.74$\pm$0.03} & \textbf{38.83$\pm$0.05} & \textbf{89.50$\pm$0.04} \\
 \midrule
\multirow{2}{*}{\begin{tabular}[c]{@{}c@{}}ViT-B/16\end{tabular}} 
    & MSP & 51.52 & 88.16 & 66.56 & 80.93 & 60.23 & 82.99 & 68.68 & 80.38 & 61.75 & 83.12 \\
    & \textbf{MSP+Ours} & \textbf{20.45$\pm$0.10} & \textbf{95.77$\pm$0.06} & \textbf{29.95$\pm$0.45} & \textbf{92.88$\pm$0.03} & \textbf{43.93$\pm$0.37} & \textbf{89.51$\pm$0.14} & \textbf{41.88$\pm$0.40} & \textbf{89.32$\pm$0.11} & \textbf{34.05$\pm$0.05} & \textbf{91.87$\pm$0.05} \\
 \midrule
 \multirow{2}{*}{\begin{tabular}[c]{@{}c@{}}ConvNext\end{tabular}} 
    & MSP & 44.69 & 89.67 & 63.47 & 79.39 & 65.83 & 73.82 & 67.06 & 78.44 & 60.26 & 80.33 \\
    & \textbf{MSP+Ours} & \textbf{23.34$\pm$0.26} & \textbf{95.06$\pm$0.10} & \textbf{31.61$\pm$0.70} & \textbf{92.18$\pm$0.20} & \textbf{60.23$\pm$0.32} & \textbf{80.76$\pm$0.16} & \textbf{43.16$\pm$0.21} & \textbf{88.60$\pm$0.09} & \textbf{39.58$\pm$0.26} & \textbf{89.15$\pm$0.12} \\
 \midrule
 \multirow{2}{*}{\begin{tabular}[c]{@{}c@{}}CLIP-RN50\end{tabular}} 
    & MCM & 33.90 & 93.72 & 48.35 & 90.42 & 61.28 & 85.29 & 60.45 & 85.90 & 51.00 & 88.83 \\
    & \textbf{MCM+Ours} & \textbf{9.45$\pm$0.23} & \textbf{98.06$\pm$0.02} & \textbf{22.69$\pm$0.17} & \textbf{95.54$\pm$0.20} & \textbf{42.79$\pm$0.06} & \textbf{90.90$\pm$0.05} & \textbf{39.63$\pm$0.21} & \textbf{90.20$\pm$0.02} & \textbf{28.64$\pm$0.05} & \textbf{93.68$\pm$0.02} \\
 \midrule
  \multirow{2}{*}{\begin{tabular}[c]{@{}c@{}}CLIP-L/14\end{tabular}} 
    & MCM & 30.14 & 94.86 & 27.63 & 94.34 & 59.27 & 84.66 & 32.34 & 92.73 & 37.35 & 91.65 \\
    & \textbf{MCM+Ours} & \textbf{7.11$\pm$0.15} & \textbf{98.28$\pm$0.01} & \textbf{14.02$\pm$0.29} & \textbf{97.23$\pm$0.07} & \textbf{47.20$\pm$1.06} & \textbf{89.79$\pm$0.11} & \textbf{24.24$\pm$0.26} & \textbf{94.29$\pm$0.03} & \textbf{23.14$\pm$0.25} & \textbf{94.90$\pm$0.02} \\
 \midrule
 \multirow{2}{*}{\begin{tabular}[c]{@{}c@{}}CLIP-B/32\end{tabular}} 
    & MCM & 41.30 & 92.82 & 44.93 & 90.93 & 62.11 & 84.78 & 47.36 & 89.31 & 48.93 & 89.46 \\
    & \textbf{MCM+Ours} & \textbf{9.28$\pm$0.14} & \textbf{98.05$\pm$0.03} & \textbf{20.65$\pm$0.07} & \textbf{96.02$\pm$0.03} & \textbf{44.08$\pm$0.44} & \textbf{90.20$\pm$0.06} & \textbf{30.24$\pm$0.24} & \textbf{92.85$\pm$0.02} & \textbf{26.06$\pm$0.16} & \textbf{94.28$\pm$0.01} \\
 
\bottomrule
\end{tabular}%
\caption{OOD detection performance with different architectures on ImageNet-1K(ID).}
\label{tab:other arch}
\end{table}

\begin{table}[!ht]
\centering
\fontsize{7}{9}\selectfont % 设置字体大小为 7pt，行距为 9pt
\setlength{\tabcolsep}{1mm}
\begin{tabular}{clccccccccccccccc}
\toprule
\multirow{3}{*}{\begin{tabular}[c]{@{}c@{}}{ID dataset}\end{tabular}} 
&\multirow{3}{*}{Method} & \multicolumn{8}{c}{OOD Datasets} & \multicolumn{2}{c}{\multirow{2}{*}{Average}} \\ \cline{3-10} 
&  & \multicolumn{2}{c}{iNaturalist} & \multicolumn{2}{c}{SUN} & \multicolumn{2}{c}{Textures} & \multicolumn{2}{c}{Places} \\
\cmidrule(lr){3-4} \cmidrule(lr){5-6} \cmidrule(lr){7-8} \cmidrule(lr){9-10} \cmidrule(lr){11-12}
& & FPR95$\downarrow$ & AUROC$\uparrow$ 
& FPR95$\downarrow$ & AUROC$\uparrow$ 
& FPR95$\downarrow$ & AUROC$\uparrow$ 
& FPR95$\downarrow$ & AUROC$\uparrow$ 
& FPR95$\downarrow$ & AUROC$\uparrow$ \\ 
\midrule

 \multirow{2}{*}{\begin{tabular}[c]{@{}c@{}}ImageNet100\end{tabular}} 
    & MCM & 12.87 & 97.30 & 36.48 & 94.64 & 37.64 & 93.34 & 32.21 & 94.78 & 30.05 & 95.02 \\
    & \textbf{MCM+Ours} & \textbf{2.32$\pm$0.09} & \textbf{99.20$\pm$0.01} & \textbf{8.93$\pm$0.02} & \textbf{98.07$\pm$0.01} & \textbf{20.75$\pm$0.12} & \textbf{96.58$\pm$0.03} & \textbf{15.15$\pm$0.29} & \textbf{96.81$\pm$0.02} & \textbf{11.79$\pm$0.09} & \textbf{97.67$\pm$0.01} \\
 \midrule
  \multirow{2}{*}{\begin{tabular}[c]{@{}c@{}}UCF101\end{tabular}} 
    & MCM & 11.85 & 97.91 & 28.62 & 94.14 & 17.77 & 96.15 & 35.28 & 91.82 & 23.28 & 95.01 \\
    & \textbf{MCM+Ours} & \textbf{6.73$\pm$0.28} & \textbf{98.53$\pm$0.04} & \textbf{21.76$\pm$0.10} & \textbf{95.49$\pm$0.02} & \textbf{15.11$\pm$0.08} & \textbf{96.68$\pm$0.02} & \textbf{29.16$\pm$0.22} & \textbf{93.26$\pm$0.03} & \textbf{18.19$\pm$0.03} & \textbf{95.99$\pm$0.01} \\
 \midrule
 \multirow{2}{*}{\begin{tabular}[c]{@{}c@{}}FGVC-Aircraft\end{tabular}} 
    & MCM & 39.11 & 91.44 & 3.23 & 99.06 & 5.57 & 98.52 & 7.78 & 97.77 & 13.92 & 96.70 \\
    & \textbf{MCM+Ours} & \textbf{32.01$\pm$0.19} & \textbf{93.34$\pm$0.04} & \textbf{2.08$\pm$0.03} & \textbf{99.32$\pm$0.01} & \textbf{3.87$\pm$0.02} & \textbf{98.94$\pm$0.02} & \textbf{6.80$\pm$0.03} & \textbf{98.04$\pm$0.02} & \textbf{11.19$\pm$0.07} & \textbf{97.41$\pm$0.01} \\
 
\bottomrule
\end{tabular}%
\caption{OOD detection performance on other ID datasets using CLIP-B/16.}
\label{tab:other_ID_details}
\end{table}

\begin{table}[!ht]
\centering
\fontsize{5.5}{9}\selectfont % 设置字体大小为 5.5pt，行距为 9pt
\setlength{\tabcolsep}{1mm}
\begin{tabular}{clcccccccccccccccc}
\toprule
\multirow{3}{*}{\begin{tabular}[c]{@{}c@{}}{ID dataset}\end{tabular}} 
&\multirow{3}{*}{Method} & \multicolumn{12}{c}{OOD Datasets} & \multicolumn{2}{c}{\multirow{2}{*}{Average}} \\ \cline{3-14} 
&  & \multicolumn{2}{c}{SVHN} & \multicolumn{2}{c}{LSUN-R} & \multicolumn{2}{c}{LSUN-C} & \multicolumn{2}{c}{iSUN} & \multicolumn{2}{c}{Textures} & \multicolumn{2}{c}{Places365} \\
\cmidrule(lr){3-4} \cmidrule(lr){5-6} \cmidrule(lr){7-8} \cmidrule(lr){9-10} \cmidrule(lr){11-12} \cmidrule(lr){13-14} \cmidrule(lr){15-16}
& & FPR95$\downarrow$ & AUROC$\uparrow$ 
& FPR95$\downarrow$ & AUROC$\uparrow$ 
& FPR95$\downarrow$ & AUROC$\uparrow$ 
& FPR95$\downarrow$ & AUROC$\uparrow$ 
& FPR95$\downarrow$ & AUROC$\uparrow$ 
& FPR95$\downarrow$ & AUROC$\uparrow$ 
& FPR95$\downarrow$ & AUROC$\uparrow$ \\ 
\midrule

 \multirow{2}{*}{CIFAR10} 
    & MCM & 3.60 & 98.84 & 8.47 & 97.84 & 5.77 & 98.33 & 12.5 & 97.31 & 20.14  & 95.61 & 40.05 & 88.21 & 15.09 & 96.02 \\
    & \textbf{MCM+Ours} & \textbf{2.34$\pm$0.02} & \textbf{99.20$\pm$0.01} & \textbf{5.44$\pm$0.03} & \textbf{98.56$\pm$0.01} & \textbf{4.28$\pm$0.01} & \textbf{98.62$\pm$0.02} & \textbf{8.74$\pm$0.02} & \textbf{97.95$\pm$0.03} & \textbf{19.75$\pm$0.10} & \textbf{95.74$\pm$0.06} & \textbf{35.81$\pm$0.13} & \textbf{88.98$\pm$0.10} & \textbf{12.73$\pm$0.05} & \textbf{96.51$\pm$0.02} \\
 \midrule
 \multirow{2}{*}{CIFAR100} 
    & MCM & 83.53 & 87.34 & 83.07 & 82.26 & 71.47 & 87.49 & 80.9 & 81.93 & 98.01 & 66.71 & 99.68 & 52.78 & 86.11 & 76.42 \\
    & \textbf{MCM+Ours} & \textbf{31.80$\pm$0.33} & \textbf{94.78$\pm$0.02} & \textbf{66.96$\pm$0.21} & \textbf{86.61$\pm$0.09} & \textbf{48.42$\pm$0.31} & \textbf{91.25$\pm$0.06} & \textbf{68.86$\pm$0.45} & \textbf{85.80$\pm$0.10} & \textbf{97.79$\pm$0.04} & \textbf{66.86$\pm$0.03} & \textbf{99.66$\pm$0.02} & \textbf{53.27$\pm$0.08} & \textbf{68.91$\pm$0.07} & \textbf{79.76$\pm$0.04} \\
\bottomrule
\end{tabular}
\caption{OOD detection performance on CIFAR benchmark using CLIP-B/16.}
\label{tab:cifar_results}
\end{table}
